# Supplementary material for: Arriving on time: estimating travel time distributions on large-scale road networks
Source: arXiv:1302.6617 source file (2013-02-26)
Supplement: Supplementary file 1 [file appendix.tex]

%!TEX root =article.tex
\appendix
%Appendix A
%\section{Appendices}
%The rules about hierarchical headings discussed above for
%the body of the article are different in the appendices.
%In the \textbf{appendix} environment, the command
%\textbf{section} is used to
%indicate the start of each Appendix, with alphabetic order
%designation (i.e. the first is A, the second B, etc.) and
%a title (if you include one).  So, if you need
%hierarchical structure
%\textit{within} an Appendix, start with \textbf{subsection} as the
%highest level. Here is an outline of the body of this
%document in Appendix-appropriate form:
%\subsection{Introduction}
%\subsection{The Body of the Paper}
%\subsubsection{Type Changes and  Special Characters}
%\subsubsection{Math Equations}
%\paragraph{Inline (In-text) Equations}
%\paragraph{Display Equations}
%\subsubsection{Citations}
%\subsubsection{Tables}
%\subsubsection{Figures}
%\subsubsection{Theorem-like Constructs}
%\subsubsection*{A Caveat for the \TeX\ Expert}
%\subsection{Conclusions}
%\subsection{Acknowledgments}
%\subsection{Additional Authors}
%This section is inserted by \LaTeX; you do not insert it.
%You just add the names and information in the
%\texttt{{\char'134}additionalauthors} command at the start
%of the document.
